# Supplementary material for: More Parameters? No Thanks!
Source: arXiv:2107.09622 source file (2021-07-20)
Supplement: Supplementary file 1 [file appendix.tex]

\begin{table}[]
    \centering
    \begin{tabular}{c|c}
         &  \\
         & 
    \end{tabular}
    \caption{Caption}
    \label{tab:my_label}
\end{table}

Ar - 214111 - 1 - 507
Az - 005946 - 7 - 27
Be - 004509 - 8 - 27 (LOL)
De - 167888 - 4 - 400
Gl - 010017 - 6 - 33
He - 211819 - 2 - 486
It - 204503 - 3 - 490
Sk - 061470 - 5 - 162
